# Supplementary material for: Adaptive Gating for Single-Photon 3D Imaging
Source: arXiv:2111.15047 source file (2022-04-11)
Supplement: Supplementary file 11 [file adaptive_supplement.tex]

% CVPR 2022 Paper Template
% based on the CVPR template provided by Ming-Ming Cheng (https://github.com/MCG-NKU/CVPR_Template)
% modified and extended by Stefan Roth (stefan.roth@NOSPAMtu-darmstadt.de)

\documentclass[10pt,onecolumn,letterpaper]{article}

%%%%%%%%% PAPER TYPE  - PLEASE UPDATE FOR FINAL VERSION
%\usepackage[review]{cvpr}      % To produce the REVIEW version
\usepackage{cvpr}              % To produce the CAMERA-READY version
%\usepackage[pagenumbers]{cvpr} % To force page numbers, e.g. for an arXiv version
\usepackage{times}
\usepackage{amsmath}
% Include other packages here, before hyperref.
\usepackage{units}
\usepackage{amsmath, amsthm, amssymb}
\usepackage{mathtools}
\usepackage{amssymb}
\usepackage{nicefrac}
\usepackage{xfrac}
\usepackage{bm}
\usepackage{mathdefs}
\usepackage{graphicx}
\usepackage{colortbl}
\usepackage{xspace}
\usepackage{booktabs}
\usepackage{caption}
\usepackage{color}
\usepackage[accsupp]{axessibility} 

\usepackage{comment}
\usepackage{algorithm}
\usepackage{algpseudocode}

% It is strongly recommended to use hyperref, especially for the review version.
% hyperref with option pagebackref eases the reviewers' job.
% Please disable hyperref *only* if you encounter grave issues, e.g. with the
% file validation for the camera-ready version.
%
% If you comment hyperref and then uncomment it, you should delete
% ReviewTempalte.aux before re-running LaTeX.
% (Or just hit 'q' on the first LaTeX run, let it finish, and you
%  should be clear).

% If you comment hyperref and then uncomment it, you should delete
% egpaper.aux before re-running latex.  (Or just hit 'q' on the first latex
% run, let it finish, and you should be clear).
\usepackage[pagebackref=true,breaklinks=true,letterpaper=true,colorlinks,bookmarks=false]{hyperref}

% Support for easy cross-referencing
\usepackage[capitalize]{cleveref}
\usepackage{adaptive_supplement}
\usepackage[figurename=Supplementary Figure]{caption}

\graphicspath{{figures/}}

%%%%%%%%% PAPER ID  - PLEASE UPDATE
\def\cvprPaperID{7228} % *** Enter the CVPR Paper ID here
\def\confName{CVPR}
\def\confYear{2022}

\begin{document}
%%%%%%%%% TITLE - PLEASE UPDATE
\title{Adaptive Gating for Single-Photon 3D Imaging: Supplementary Material}

\maketitle

\tableofcontents

\input{discussion}
%\newpage
\input{code}
%\newpage  
\input{experimental_details}
%\newpage  
\input{adaptive_exposure}
%\newpage
\input{estimators_and_lower_exposures}
%\newpage 
\input{dead_time_effects}
%\newpage
\input{per_pixel_entropy}
%\newpage
\input{model_mismatch}
%\newpage 
\input{additional_figures}
%\newpage

%%%%%%%%% REFERENCES
{\small
\bibliographystyle{ieee_fullname}
\bibliography{adaptive_supplement}
}
\end{document}
